# Supplementary material for: Introduction to Engineering Mathematics and Analysis: Modeling Physical Systems Using the Language of Mathematics
Source: arXiv:2305.05036 source file (2023-05-08)
Supplement: Supplementary file 1 [file solution_first_order_wave_Laplace.pdf]

$$\frac{\partial u}{\partial t} = -c\frac{\partial u}{\partial x} \qquad -\infty < x < \infty$$

$$u(x,0) = e^{-x}H(x)$$

---

$$sU - e^{-x}H(x) = -c\frac{dU}{dx}$$

$$\frac{dU}{dx} + \frac{s}{c}U = \frac{1}{c}e^{-x}H(x)$$

$$\frac{d}{dx}\left(Ue^{\frac{s}{c}x}\right) = \frac{1}{c}e^{\frac{s}{c}x}e^{-x}H(x)$$

$$\int_{-\infty}^{x}\frac{dU}{dx}e^{s/c}\,dx = \frac{1}{c}\int_{-\infty}^{x}e^{\left(\frac{s}{c}-1\right)z}H(z)\,dz$$

$$U(x,s)e^{s/c\,x} = \frac{1}{c}\int_{-\infty}^{\infty}\exp\left[-z\left(1-\frac{s}{c}\right)\right]H(z)\,dz$$

$$U(x,s) = \frac{e^{-\frac{s}{c}x}}{c}\int_{0}^{\infty}\exp\left[-z\left(1-\frac{s}{c}\right)\right]dz$$

$$= \left(\frac{e^{-\frac{s}{c}x}}{c}\right)\left(-\frac{1}{1-\frac{s}{c}}\exp\left(-z\left(1-\frac{s}{c}\right)\right)\right)\Bigg|_{0}^{\infty}$$

$$U(x,s) = \frac{1}{c}\int_0^\infty \exp\left[-\frac{s}{c}x + \frac{s}{c}z - z\right] dz$$

$$= \frac{1}{c}\int_0^\infty \exp\left[-\frac{s}{c}(x - z)\right] x$$

$$= \frac{1}{c}\int_0^\infty \exp\left[-\frac{s}{c}x + z\left(\frac{s}{c} - 1\right)\right]$$

$$\frac{s}{c}x > z\left(1 - \frac{s}{c}\right)$$

$$x > z\left(\frac{c}{s} - 1\right)$$

$$= \frac{1}{c}\int \exp\left[-\frac{s}{c}(x - z)\right]\exp(-z)$$

$x > z$

convergent

---

$$H \exp\left(-\frac{s}{c}x\right) \; [illegible] \; \exp\left(z\left(\frac{s}{c} - 1\right)\right)$$

$\frac{s}{c} - 1$

$$e^{-x}H(x) \to e^{-(x-ct)}H(x-ct)$$

Rewrite as

$$= \frac{1}{c}\exp\left(-\frac{s}{c}x\right)\int_0^x \exp\left(z\left(\frac{s}{c}-1\right)\right)dz$$

$$= \left[\frac{1}{c}\exp\left(-\frac{s}{c}x\right)\right]\left[\frac{1}{\frac{s}{c}-1}\exp\left(z\left(\frac{s}{c}-1\right)\right)\right]_0^x$$

$$= \frac{1}{c}\exp\left(-\frac{s}{c}x\right)\frac{c}{s-c}\left\{\exp\left(x\left(\frac{s}{c}\right)\right)\exp(-x) - 1\right\}$$

$$= \frac{1}{s-c}\exp(-x) - \frac{\exp\left(-\frac{s}{c}x\right)}{(s-c)}$$

Answer should be

$$\frac{1}{s-c}e^{-x} - \frac{1}{s-c}e^{-sx/c}$$ invert →

exp(
